# Supplementary material for: Ternary MobileNets via Per-Layer Hybrid Filter Banks
Source: arXiv:1911.01028 source file (2019-11-04)
Supplement: Supplementary file 1 [file quant_impact_on_float16.tex]

\section{Changes in Full-Precision Filter Values After Applying Quantization.}
\label{sec:quant_impact_on_float16}
\begin{figure}[!tbp]
  \centering
  \subfloat[A MobileNets layer with hybrid filter bank.]{\includegraphics[width=0.4\textwidth]{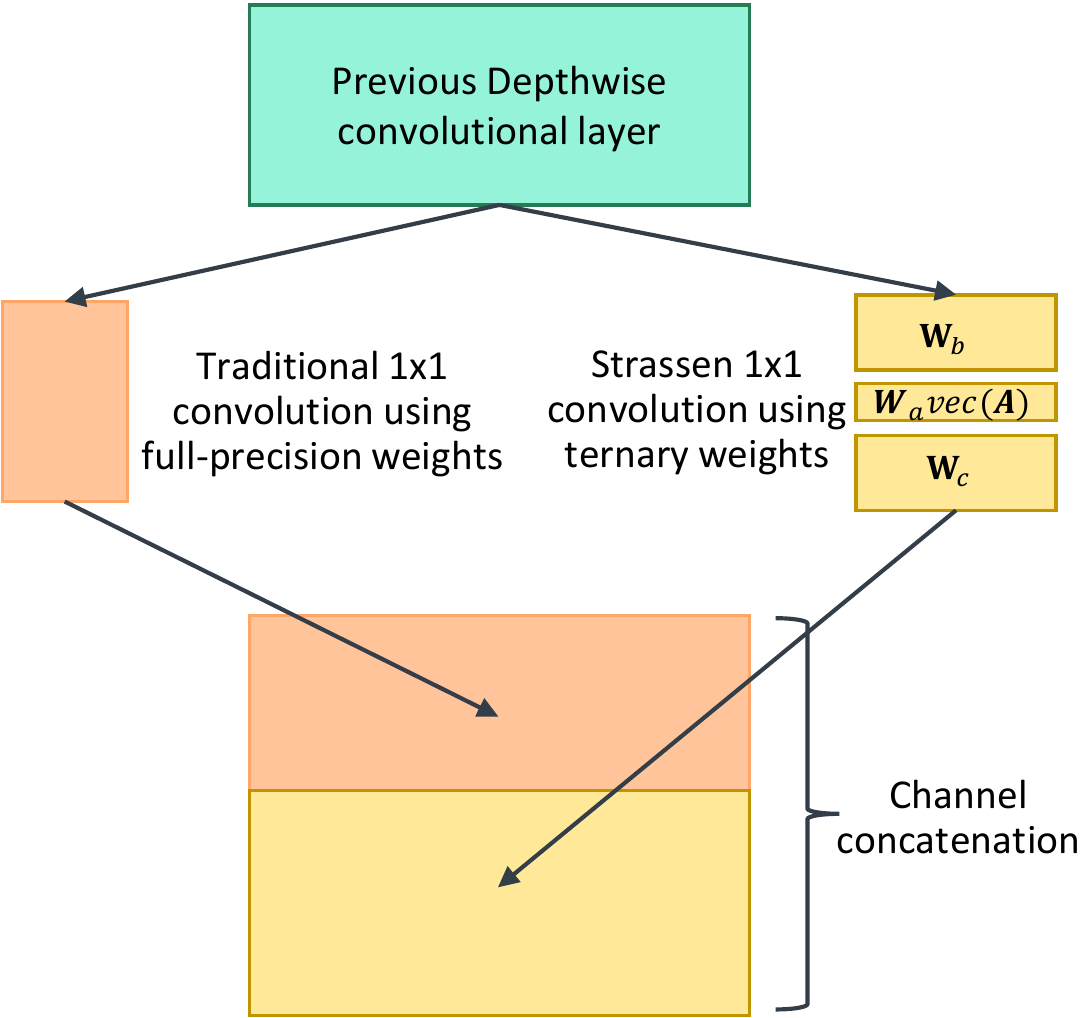}\label{fig:hybrid_1x1_filter_bank}}
  \hfill
  \subfloat[Inception module from GoogleNet.]{\includegraphics[width=0.4\textwidth]{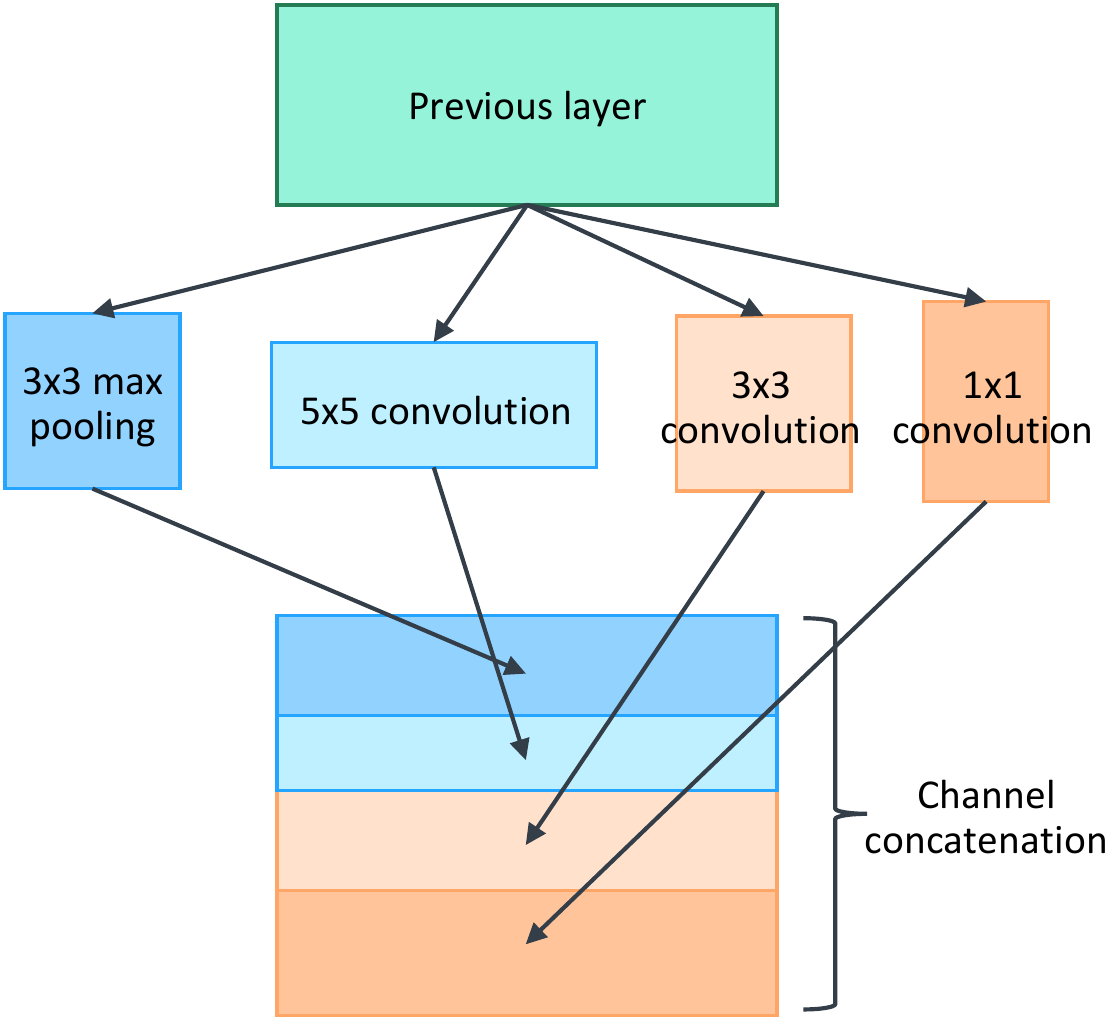}\label{fig:inception_module}}
  \caption{MobileNets with hybrid filter banks and its relation to Inception module from GoogleNet.}
  \label{fig:quant_impact_on_float16}
\end{figure}

For each full-precision convolutional filter of a hybrid filter bank, we measure the L2 distance of its weight values before and after quantization is applied over the overall Hybrid MobileNets architecture. Figure~\ref{fig:quant_impact_on_float16} shows the bell curve of the L2 distances of filter weights for first few layers of Hybrid MobileNets. It is confirmed from the bell curves that during the quantization phase, few full-precision filters at each hybrid filter bank change significantly while other change moderately. This in turn corroborates the fact that 
during the quantization-aware training phase, the organization of hybrid filter banks influences the filters that require full-precision values to extract features to be trained using traditional convolutions, and the filters that are less susceptible to ternary quantization to be trained using ternary values from strassenified convolutions.
